# Supplementary material for: Visible Light Indoor Positioning with a Single LED and Distributed Single-Element OIRS: An Iterative Approach with Adaptive Beam Steering
Source: arXiv:2507.14148 source file (2025-12-16)
Supplement: Supplementary file 1 [file Supplementary_Materials.pdf]

# SUPPLEMENTARY MATERIAL FOR

## VISIBLE LIGHT INDOOR POSITIONING WITH A SINGLE LED AND DISTRIBUTED SINGLE-ELEMENT OIRS: AN ITERATIVE APPROACH WITH ADAPTIVE BEAM STEERING

D. PUGLIESE, G. IACOVELLI, A. FASCISTA, D. STRICCOLI, O. ROMANOV,  
L. A. GRIECO, G. BOGGIA

### S-I. REFLECTION POINT GEOMETRIC MODEL

We derive the geometric model of the reflection point  $\mathbf{r}_n$ , relating it to the Light Emitting Diode (LED), Photo Detector (PD), and the  $n$ -th Optical Intelligent Reflective Surface (OIRS). Let  $\mathcal{R}_x(\cdot)$ ,  $\mathcal{R}_y(\cdot)$ , and  $\mathcal{R}_z(\cdot)$  denote counterclockwise rotations about the  $x$ ,  $y$ , and  $z$  axes. To compute  $\mathbf{r}_n$ , we translate the reference frame so that it is centered at  $\mathbf{w}_n$ , with the  $z$ -axis oriented downward, the  $x$ -axis aligned parallel to the ground, and the  $y$ -axis pointing outward from the OIRS, as shown in Fig. S-1. A generic point  $\mathbf{p} = [p_x \ p_y \ p_z]^T$  in the local coordinate system  $O(x'y'z')$  centered at the  $n$ -th OIRS can be expressed as

$$\mathbf{p}' = \begin{cases} \mathcal{R}_y(\pi)\mathcal{R}_z(3\pi/2)(\mathbf{p} - \mathbf{w}_n), & \text{if } \mathbf{o}_n = (1, 0, 0), \\ \mathcal{R}_y(\pi)(\mathbf{p} - \mathbf{w}_n), & \text{if } \mathbf{o}_n = (0, 1, 0), \\ \mathcal{R}_y(\pi)\mathcal{R}_z(\pi)(\mathbf{p} - \mathbf{w}_n), & \text{if } \mathbf{o}_n = (-1, 0, 0), \\ \mathcal{R}_y(\pi)\mathcal{R}_z(\pi/2)(\mathbf{p} - \mathbf{w}_n), & \text{if } \mathbf{o}_n = (0, -1, 0), \end{cases} \quad (\text{S1})$$

where we recall  $\mathbf{o}_n$  is the unit vector associated with the initial orientation of the  $n$ -th OIRS. The positions of the LED, the reflection point, the center of the OIRS, and the PD in the new reference frame are denoted as  $\mathbf{q}' = [q'_x \ q'_y \ q'_z]^T$ ,  $\mathbf{r}' = [r'_x \ 0 \ r'_z]^T$ ,  $\mathbf{w}' = [0 \ 0 \ 0]^T$ , and  $\mathbf{u}' = [u'_x \ u'_y \ u'_z]^T$ , respectively, where from now on we drop the dependency on  $n$  for brevity. Accordingly, we define  $s = \|\mathbf{q}' - \mathbf{r}'\|$  as the distance from the LED to the reflection point, where  $\theta^{\text{IN}}$  and  $\varphi^{\text{IN}}$  denote the corresponding azimuth and elevation angles of incidence. Similarly,  $d = \|\mathbf{r}' - \mathbf{u}'\|$  represents the distance from the reflection point to the PD, with  $\theta^{\text{IR}}$  and  $\varphi^{\text{IR}}$  denoting the azimuth and elevation angles of irradiance, respectively, as illustrated in Fig. S-1. This formulation naturally extends when the OIRS orientation is adjusted: the rotations in (S1) are further composed with a transformation defined by  $\mathcal{R}_x(\beta_n)\mathcal{R}_z(\alpha_n)$ , where we recall  $\beta_n$  and  $\alpha_n$  represent the OIRS control angles around the  $x$  and  $z$  axes, respectively.

Using polar coordinates,  $\mathbf{u}'$  can be expressed as

$$\begin{cases} u'_x = r'_x - d \sin(\theta^{\text{IR}}) \cos(\varphi^{\text{IR}}), \\ u'_y = d \sin(\theta^{\text{IR}}) \sin(\varphi^{\text{IR}}), \\ u'_z = r'_z + d \cos(\theta^{\text{IR}}), \end{cases} \quad (\text{S2})$$

with  $d = |\mathbf{u}'_z - r'_z| / \cos(\theta^{\text{IR}})$  and, without loss of generality,  $r'_x < 0$ . By plugging these values back in (S2) and imposing Snell's law (i.e.,  $\theta^{\text{IR}} = \theta^{\text{IN}}$  and  $\varphi^{\text{IR}} = \varphi^{\text{IN}}$ ), we obtain

$$\begin{cases} u'_x = r'_x - \frac{\sqrt{(q'_x - r'_x)^2} \sqrt{(u'_z - r'_z)^2}}{\sqrt{(q'_z - r'_z)^2}}, \\ u'_y = \frac{\sqrt{q_y'^2} \sqrt{(u'_z - r'_z)^2}}{\sqrt{(q'_z - r'_z)^2}}, \\ u'_z = r'_z + \sqrt{(u'_x - r'_x)^2}, \end{cases} \quad (\text{S3})$$

with

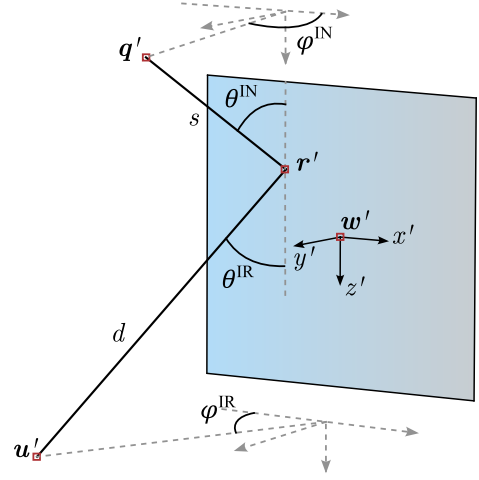

Fig. S-1. Geometric representation of the reflection point on the OIRS surface.

$$\begin{aligned} \cos(\theta^{\text{IN}}) &= \frac{\sqrt{(q'_z - r'_z)^2}}{\|\mathbf{q}' - \mathbf{r}'\|}, & \sin(\theta^{\text{IN}}) &= \frac{\sqrt{(q'_x - r'_x)^2 + q_y'^2}}{\|\mathbf{q}' - \mathbf{r}'\|} \\ \cos(\varphi^{\text{IN}}) &= \frac{\sqrt{(q'_x - r'_x)^2}}{\sqrt{(q'_x - r'_x)^2 + q_y'^2}}, & \sin(\varphi^{\text{IN}}) &= \frac{\sqrt{q_y'^2}}{\sqrt{(q'_x - r'_x)^2 + q_y'^2}}. \end{aligned}$$

The final expression of  $\mathbf{r}'$  follows by solving (S3), namely

$$r'_x = \frac{q'_x u'_y + q'_y u'_x}{q'_y + u'_y}, \quad r'_z = \frac{q'_y u'_z + q'_z u'_y}{q'_y + u'_y}. \quad (\text{S4})$$

The transformations in (S1) can be then applied in the opposite way to map  $\mathbf{r}'$  back to the global reference system.

### S-II. DERIVATION OF RML NLOS DISTANCE ESTIMATOR

We start by expanding the expression of the compressed likelihood function in (35) and by applying a change of variable  $z(d_n) = \frac{1}{(s_n + d_n)^2 d_n}$ , so that

$$\tilde{\mathcal{L}}^{\text{NLoS}}(\chi_n; d_n) = T_2 - 2T_1 \omega z(d_n) + \omega^2 z^2(d_n), \quad (\text{S5})$$

where we introduced the summation terms

$$T_1 = \frac{1}{K_n} \sum_{k=1}^{K_n} \chi_{n,k}, \quad T_2 = \frac{1}{K_n} \sum_{k=1}^{K_n} \chi_{n,k}^2. \quad (\text{S6})$$

To find the minimum, we then derive  $\tilde{\mathcal{L}}^{\text{NLoS}}(\chi_n; d_n)$  wrt  $d_n$  and set it to zero

$$\begin{aligned} \frac{\partial \tilde{\mathcal{L}}^{\text{NLoS}}(\chi_n; d_n)}{\partial d_n} &= (-2T_1 \omega + 2\omega^2 z(d_n)) \frac{\partial z(d_n)}{\partial d_n} = 0 \\ \Rightarrow z(d_n) &= \frac{1}{(s_n + d_n)^2 d_n} = \frac{T_1}{\omega} \\ \Rightarrow d_n^3 + 2s_n d_n^2 + s_n^2 d_n - \frac{\omega}{T_1} &= 0. \end{aligned} \quad (\text{S7})$$

We then apply the substitution  $d_n = t - \frac{2s_n}{3}$  to reduce (S7) to a depressed cubic  $t^3 + \kappa t + \iota = 0$  (with  $\kappa$  and  $\iota$  depending on  $s_n$ ,  $\omega$ , and  $T_1$ ). The closed-form solution in (37) follows by applying Cardano's formula to the depressed cubic equation and retaining the unique real solution among the three roots.

### S-III. ENTRIES OF FIM IN (51)

We consider the log-likelihood of (50), which is

$$\ln L(\boldsymbol{\mu}; \mathbf{d}) = \mathcal{L}^{\text{LoS}}(\boldsymbol{\mu}_0; d) + \sum_{n=1}^N \mathcal{L}^{\text{NLoS}}(\boldsymbol{\mu}_n; d, d_n), \quad (\text{S8})$$

where  $\mathcal{L}^{\text{LoS}}(\boldsymbol{\mu}_0; d)$  and  $\mathcal{L}^{\text{NLoS}}(\boldsymbol{\mu}_n; d, d_n)$  are recast as the positive form of (16) and (31). The first step to compute each element of the Fisher Information Matrix (FIM) in (51) involves computing the relevant partial derivatives which, owing to the additive structure of (S8), can be performed separately for the Line-of-Sight (LoS) and Non-Line-of-Sight (NLoS) components of the log-likelihood. To facilitate the upcoming derivations, we define the following summation terms

$$\begin{aligned} \mathcal{S}_0 &= \sum_{k=1}^K \left( \mu_{0,k} - \frac{\xi}{d^{m+3}} \right), \quad \mathcal{T}_0 = \sum_{k=1}^K \left( \mu_{0,k} - \frac{\xi}{d^{m+3}} \right)^2, \\ \mathcal{S}_n &= \sum_{k=1}^{K_n} \left( \mu_{n,k} - \frac{\xi}{d^{m+3}} - \frac{\omega}{d_n(d_n + s_n)^2} \right), \\ \mathcal{T}_n &= \sum_{k=1}^{K_n} \left( \mu_{n,k} - \frac{\xi}{d^{m+3}} - \frac{\omega}{d_n(d_n + s_n)^2} \right)^2. \end{aligned} \quad (\text{S9})$$

As for the  $(0, 0)$ -th element of  $\mathbf{J}_d$ , the derivatives of the LoS and the  $n$ -th NLoS parts,  $\forall n = 1, \dots, N$ , are given by

$$\begin{aligned} \frac{\partial^2 \mathcal{L}^{\text{LoS}}(\boldsymbol{\mu}_0; d)}{\partial d \partial d} &= \frac{\bar{\mu}_0(m^2 + 7m + 12) \left( \frac{b}{\sigma_0^2} \mathcal{T}_0 + 2\mathcal{S}_0 - bK \right)}{2d^2 \sigma_0^2} \\ &- \frac{\bar{\mu}_0^2(m+3)^2 \left( \frac{b^2}{\sigma_0^2} \mathcal{T}_0 + 2b\mathcal{S}_0 + K \left( \sigma_0^2 - \frac{b^2}{2} \right) \right)}{d^2 \sigma_0^4}, \quad (\text{S10}) \\ \frac{\partial^2 \mathcal{L}^{\text{NLoS}}(\boldsymbol{\mu}_n; d, d_n)}{\partial d \partial d} &= \frac{\bar{\mu}_0(m^2 + 7m + 12) \left( \frac{b}{\sigma_0^2} \mathcal{T}_n + 2\mathcal{S}_n - bK_n \right)}{2d^2 \sigma_0^2} \\ &- \frac{\bar{\mu}_0^2(m+3)^2 \left( \frac{b^2}{\sigma_0^2} \mathcal{T}_n + 2b\mathcal{S}_n + K_n \left( \sigma_0^2 - \frac{b^2}{2} \right) \right)}{d^2 \sigma_0^4}. \end{aligned}$$

For the  $(n, n)$ -th diagonal entries of  $\mathbf{J}_d$ , only the derivative of the log-likelihood term associated with the  $n$ -th NLoS component is non-zero, and it is given by

$$\begin{aligned} \frac{\partial^2 \mathcal{L}^{\text{NLoS}}(\boldsymbol{\mu}_n; d, d_n)}{\partial d_n \partial d_n} &= \\ &\frac{\bar{\chi}_n(6d_n^2 + 4d_n s_n + s_n^2) \left( \frac{b}{\sigma_n^2} \mathcal{T}_n + 2\mathcal{S}_n - bK_n \right)}{d_n^2 \sigma_n^2 (d_n + s_n)^2} \\ &- \frac{\bar{\chi}_n^2(3d_n + s_n)^2 \left( \frac{b^2}{\sigma_n^2} \mathcal{T}_n + 2b\mathcal{S}_n + K_n \left( \sigma_n^2 - \frac{b^2}{2} \right) \right)}{d_n^2 \sigma_n^4 (d_n + s_n)^2}. \end{aligned} \quad (\text{S11})$$

A similar consideration holds for the  $(0, n)$ -th element, which is equal to the symmetric  $(n, 0)$ -th entry, resulting in

$$\begin{aligned} \frac{\partial^2 \mathcal{L}^{\text{NLoS}}(\boldsymbol{\mu}_n; d, d_n)}{\partial d \partial d_n} &= \frac{\partial^2 \mathcal{L}^{\text{NLoS}}(\boldsymbol{\mu}_n; d, d_n)}{\partial d_n \partial d} = \\ &- \frac{\bar{\mu}_n \bar{\chi}_n(m+3)(3d_n + s_n) \left( \frac{b^2}{\sigma_n^2} \mathcal{T}_n + 2b\mathcal{S}_n + K_n \left( \sigma_n^2 - \frac{b^2}{2} \right) \right)}{dd_n \sigma_n^4 (d_n + s_n)}. \end{aligned} \quad (\text{S12})$$

All other elements are zero. We can now take the negative expectation of each element which, when applied to the summations (S9) appearing in (S10), (S11), and (S12), yields

$$\begin{aligned} \mathbb{E}[\mathcal{S}_0] &= 0, \quad \mathbb{E}[\mathcal{S}_n] = 0, \\ \mathbb{E}[\mathcal{T}_0] &= K \left( a + b \left( \frac{\xi}{d^{m+3}} \right) \right) = K \sigma_0^2, \\ \mathbb{E}[\mathcal{T}_n] &= K_n \left( a + b \left( \frac{\xi}{d^{m+3}} + \frac{\omega}{d_n(d_n + s_n)^2} \right) \right) = K_n \sigma_n^2. \end{aligned} \quad (\text{S13})$$

Therefore, we finally obtain

$$[\mathbf{J}_d]_{0,0} = -\mathbb{E} \left[ \frac{\partial^2 \ln L(\boldsymbol{\mu}; \mathbf{d})}{\partial d \partial d} \right] = \quad (\text{S14})$$

$$\begin{aligned} &J_d + \sum_{n=1}^N \left( \frac{K_n \bar{\mu}_0^2(m+3)^2(\sigma_n^2 + b^2/2)}{d^2 \sigma_n^4} \right), \\ [\mathbf{J}_d]_{0,n} &= [\mathbf{J}_d]_{n,0} = -\mathbb{E} \left[ \frac{\partial^2 \ln L(\boldsymbol{\mu}; \mathbf{d})}{\partial d_n \partial d} \right] = \\ &\frac{K_n \bar{\mu}_0(m+3) \bar{\chi}_n(b^2 + 2\sigma^2)(3d_n + s_n)}{2dd_n \sigma_n^4 (d_n + s_n)}, \end{aligned} \quad (\text{S15})$$

$[\mathbf{J}_d]_{n,n} = J_{d_n}$ , and  $[\mathbf{J}_d]_{n,n'} = 0$  for  $n \neq n' \neq 0$ . As it can be observed,  $[\mathbf{J}_d]_{n,n}$  has the same structure as the NLoS Fisher information in (48), while the first element of the summation in (S14) reflects the LoS Fisher information in (46).
